# Supplementary material for: Dynamical stability of 2D topological lasers
Source: arXiv:1912.03911 source file (2019-12-09)
Supplement: Supplementary file 1 [file appendix_A.tex]

\appendix

\chapter{Appendix AA}
\label{appendixAA}

We recall the linearized equation:
\begin{equation}\label{eq:2.5}
     -J\big[\delta \psi_{m+1,n} + \delta \psi_{m-1,n} + e^{-2\pi i \theta m} 
     \delta \psi_{m,n+1} 
      + e^{+2\pi i \theta m}\delta \psi_{m,n-1}\big] + i\big[\chi P^{eff}_{m,n} - \gamma\big] \delta \psi_{m,n} = w \delta \psi_{m,n}    
\end{equation}
with $P^{eff}_{m,n} = \frac{R P_{m,n}}{\gamma_R}$ and $\chi = (1-i\frac{g_R}{R})$

Then, about the boundary conditions, we consider 2 cases: open boundary conditions along the 2 axes, and periodic boundary condition along the $y$-axis and open along the $x$ one. In the last case, it implies adding extra terms in the treatment of system of equations (\ref{eq:2.5}), that will be denoted in {\color{blue}blue}.

Turning it into a matricial form by taking $j= m N_y + n$, the problem becomes:

\begin{equation}

    \left[
    \begin{array}{c|c|c|c|c|c}
    A_0 & -J\mathbb{1}_{N_y,N_y} & 0 & \ldots & \ldots & 0 \\
    \hline
    -J\mathbb{1}_{N_y,N_y}  & A_1 & -J\mathbb{1}_{N_y,N_y} & \ddots & & \vdots\\
    \hline
    0 & -J\mathbb{1}_{N_y,N_y} & A_2 & -J\mathbb{1}_{N_y,N_y} & \ddots & \vdots\\
    \hline
    \vdots & \ddots & \ddots & \ddots & \ddots & 0\\
    \hline
    \vdots &  & \ddots & \ddots & \ddots &  -J\mathbb{1}_{N_y,N_y}\\
    \hline
    0 & \ldots & \ldots  & 0 & -J\mathbb{1}_{N_y,N_y} & A_{N_x-1}   
    \end{array}
    \right]
          \begin{pmatrix} 
        [\delta \psi_{0,n}] \\ 
        [\delta \psi_{1,n}] \\
        [\delta \psi_{2,n}] \\ 
        ... \\  
        ...  \\
        ...  \\
        [\delta \psi_{N_x-1,n}]
      \end{pmatrix}  
      = \omega
          \begin{pmatrix} 
        [\delta \psi_{0,n}] \\ 
        [\delta \psi_{1,n}] \\
        [\delta \psi_{2,n}] \\ 
        ... \\  
        ...  \\
        ...  \\
        [\delta \psi_{N_x-1,n}]
      \end{pmatrix}
\end{equation}

\vspace{0.5 cm}

where 

\vspace{0.5 cm}

$A_m = \begin{pmatrix}
        i(\chi P^{eff}_{m,n} - \gamma) & -J e^{-2\pi i \theta (m+1)} & 0 & \ldots & 0 & {\color{blue}-J e^{+2\pi i \theta (m+1)}}\\
        -J e^{+2\pi i \theta (m+1)} & i(\chi P^{eff}_{m,n} - \gamma) & -J e^{-2\pi i \theta (m+1)} & \ddots &  &  0\\
        0 & -J e^{+2\pi i \theta (m+1)} & i(\chi P^{eff}_{m,n} - \gamma) & -J e^{-2\pi i \theta (m+1)} & \ddots & \vdots\\
        \vdots & \ddots & \ddots & \ddots & \ddots & 0\\
        0 &   & \ddots & \ddots & \ddots & -J e^{-2\pi i \theta (m+1)}\\        
        {\color{blue}-J e^{-2\pi i \theta (m+1)}} & 0 & \ldots & 0 & -J e^{+2\pi i \theta (m+1)} & i(\chi P^{eff}_{m,n} - \gamma)
\end{pmatrix}$    

of size $N_y \times N_y$.

\vspace{0.75 cm}

and $[\delta \psi_{m,n}] =           
\begin{pmatrix} 
        \delta \psi_{m,0} \\
        \delta \psi_{m,1} \\
        \delta \psi_{m,2} \\ 
        ... \\  
        ...  \\
        ...  \\
        \delta \psi_{m,N_y-1}
      \end{pmatrix}$ of size $N_y$.
