# Supplementary material for: Dynamical stability of 2D topological lasers
Source: arXiv:1912.03911 source file (2019-12-09)
Supplement: Supplementary file 2 [file appendix_B.tex]

\begin{appendices}

\chapter{Appendix BB}
\label{appendixBB}

We have the set of equations:

\begin{equation}
\begin{split}
    i\frac{\partial \delta \psi_{m,k}(t)}{\partial t} = -J[\delta \psi_{m+1,k} +  \delta \psi_{m-1,k} + 2cos(2\pi \theta m +  k_{y,0} + k) \delta \psi_{m,k}] + g\psi^0_m \ ^2 \delta \psi^*_{m,-k} \\
    +[2g|\psi^0_m|^2 + g_R N_m^0 - \mu + i(R N^0_m - \gamma)  ]\delta \psi_{m,k} + [g_R \psi_m^0 + iR \psi^0_m ]\delta N_{m,k}
\end{split}
\end{equation}

and 

\begin{equation}
 \centering
      \frac{\partial \delta N_{m,k}}{\partial t} = - (\gamma_R + R|\psi^0_{m}|^2)\delta N_{m,k} + iR N^0_m ( \psi^0_m \delta \psi^*_{m,-k} + \psi^0^*_m \delta \psi_{m,k})
\end{equation}

which can be rewritten in the matricial form:

\begin{equation}\label{eq:3.7}
    i\frac{\partial }{\partial t}
          \begin{pmatrix} 
        \delta \psi_{0,k} \\ 
        \delta \psi^*_{0-k} \\
        \delta N_{0,k}\\
        \delta \psi_{1,k} \\ 
        \delta \psi^*_{1,-k} \\ 
        \delta N_{1,k}\\
        \vdots  \\
        \vdots  \\
        \vdots  \\
        \vdots
      \end{pmatrix}
      =
      \begin{pmatrix}
      \begin{array}{lll|ccc|ccc|r}
      A_{0,k} & B_0 & C_0 &  -J & 0 & 0 &  &  & & \\
      D_{0} & E_{0,k} & F_{0} &  0 & +J & 0 &  & 0 & & \ldots\\
      G_{0} & H_{0} & I_{0}  &  0 & 0 & 0 &  &  & & \\
      \hline
      -J & 0 & 0 & A_{1,k} & B_1 & C_1 &  -J & 0 & 0& \\
      0 & +J & 0 & D_{1} & E_{1,k} & F_{1} & 0 & +J & 0& \ldots\\
      0 & 0 & 0 & G_{1} & H_{1} & I_{1,k}  & 0 & 0 &0& \\
      \hline
       &  &  & -J & 0 & 0 & \ddots & \ddots & \ddots& \ddots\\
       & 0 &  & 0 & +J & 0 & \ddots & \ddots & \ddots& 0\\
       &  &  & 0 & 0 & 0& \ddots& \ddots& \ddots& 0\\  
       \hline
        & \vdots & & & \vdots& & \ddots & 0& 0& \ddots
    \end{array}
      \end{pmatrix}
                \begin{pmatrix} 
        \delta \psi_{0,k} \\ 
        \delta \psi^*_{0-k} \\
        \delta N_{0,k}\\
        \delta \psi_{1,k} \\ 
        \delta \psi^*_{1,-k} \\ 
        \delta N_{1,k}\\
        \vdots  \\
        \vdots  \\
        \vdots  \\
        \vdots
      \end{pmatrix}
\end{equation}

where $A_{m,k} = 2g|\psi^0_m|^2 + g_R N^0_m-\mu - 2 J cos(k_{y,0} + k + 2\pi \theta m) + i(R N^0_m - \gamma)$, 

$B_m = g(\psi^0_m)^2$, 

$C_m = g_R \psi^0_m + iR\psi^0_m$, 

$D_m= -g(\psi^0_m)^{*^2}$, 

$E_{m,k} = -2g|\psi^0_m|^2 - g_R N^0_m +\mu_T + 2 J cos(k_{y,0} + k + 2\pi \theta m) + i(R N^0_m - \gamma)$, 

$F_m = -g_R \psi^0_m + iR\psi^0_m$,

$G_m = -iR N^0_m \psi^0^*$,

$H_m = -iR N^0_m \psi^0$,

$I_m = -i(R|\psi^0_m|^2 + \gamma_R)$

\end{appendices}
